# Supplementary material for: FRETtranslator: translating FRET traces into RNA structural pathways
Source: arXiv:1610.00340 source file (2016-10-02)
Supplement: Supplementary file 1 [file SuppV1.pdf]

## S1 RNA folding landscapes and basin hopping graphs

Given an RNA sequence, we consider the *underlying structural space* as the set of all secondary structures that can be formed by this sequence assuming that 1) only canonical (GC, AU, and GU) base pairs are formed, 2) hairpin loops have a minimum length of three and 3) particular types of pseudoknots defined in [33], can be included. The (free) energy $f(x)$ of each structure $x$ is a sum over binding energies of stacks and entropic contributions from unbound sections of the RNA chain. For details of the energy calculations, we refer to the literature [34]. RNA structures in the underlying structural space are arranged as a graph by specifying which pairs of structures can be interconverted in a single step, i.e., by adding or removing a base pair. This graph together with the energy function $f$ is referred to as the RNA folding landscape or simply *landscape* throughout.

Exact folding landscapes can be described easily for short RNA molecules up to around 30-nt in length. However, for longer sequences the exponential growth [35] of the underlying state space, i.e. the number of alternative structures, requires restricting the analysis to a subset of the folding landscape. For this purpose, so-called macro states or “basins” were introduced in [36], each of which represents a local minimum (LM) together with all structures that are connected to it by a gradient walk. A LM refers to the secondary structure whose energy is strictly less than the energies of all its neighboring structures in the landscape. The LM serves as the natural representative of its basin because all other structures in the same basin may refold into the LM without an energy barrier.

An “energetically favorable” neighborhood relation between such macro states is introduced in [28] and based on this relation a coarse grained model, the basin hopping graph (BHG), of the RNA folding landscape is developed. To be precise, consider two LMs $x$ and $y$ and a path $P$ connecting them in the landscape. We call a structure of maximal energy along $P$ a peak. A saddle point between $x$ and $y$ is a peak along a particular path from $x$ to $y$ with minimal possible energy. The energy of this saddle point is referred to as the saddle height between $x$ and $y$. We say that $P$ is a direct path between $x$ and $y$ if $P$ contains a peak s such that the energy is non-decreasing along $P$ from $x$ to $s$ and non-increasing from $s$ to $y$. A direct path is energetically optimal if the peak is a saddle point between $x$ and $y$ and thus if the

direct path is an energetically optimal connection between $x$ and $y$. The edges of the BHG are defined to be these energetically optimal connections. The weights on the edges reflect the corresponding saddle height and thus measure the difficulty of these favorable transitions. In this abstraction, optimal folding pathways are represented as sequences of adjacent basins represented by their LMs. The BHG is particularly suitable to describe the ruggedness of RNA folding landscapes and to explain the interconversion between multiple "active" LMs as observed in [37]. BHGs can be constructed using an efficient and accurate heuristic approach introduced in [28, 29]. This approach is feasible for RNA molecules with a length up to around 200 nt, using the energy function implemented in the ViennaRNA package [38].

FRETtranslator utilizes the resulting BHG to obtain the hidden states, initial and transition probabilities. The hidden states are the nodes in the BHG, i.e. secondary structures that are LMs represent their corresponding basins. The transition probabilities between each pair of LMs are estimated by the matrix exponential $e^{tM}$ introduced in the previous paragraph. The initial probabilities for the LMs are estimated from their Boltzmann weights. To be precise, for an LM $x$ with free energy $f(x)$ as implemented in the ViennaRNA package [38], its initial probability is $\frac{e^{-f(x)/RT}}{\sum_{s\in X} e^{-f(s)/RT}}$, where the denominator sums over all nodes s in the BHG. In the following, we refer to these LMs on the BHG as candidate structures.

## S2 Measuring the in silico inter-fluorophore distance with Ernwin

Jing Qin 7/7/2016 22:24
**Comment [1]:** PeterK: could you have again a look at this, make sure it is the updated one?

To calculate the emission probabilities of our hidden markov model, we used Ernwin to calculate inter-flourophore distances for ensembles of tertiary structures. Multitudes of tertiary structures were generated for each secondary structure (corresponding to a hidden node). Ernwin represents the tertiary structure of RNA as a set of cylinders and line segments, corresponding to the stem and loop regions, respectively. To calculate inter-nucleotide distances, the nucleotide positions are first interpolated onto the coarse grain structure as shown in S2 Fig 1.. When tested on known structures, the estimated inter-flourophore distances were strongly correlated with the distances calculated when using an all-atom model (Correlation coefficient of 0.91, See S2 Fig 2).

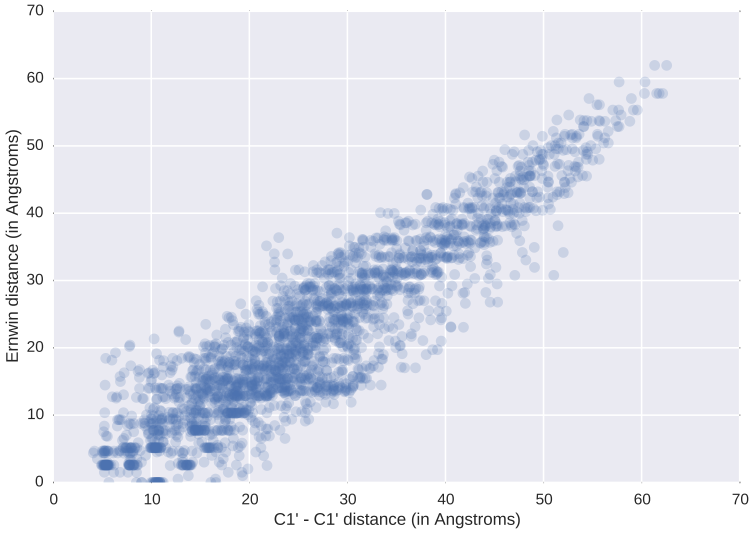


**S2 Fig 1 The inter-flourophore distances as calculated using the C1' atom distance and the estimated Ernwin position distance.**

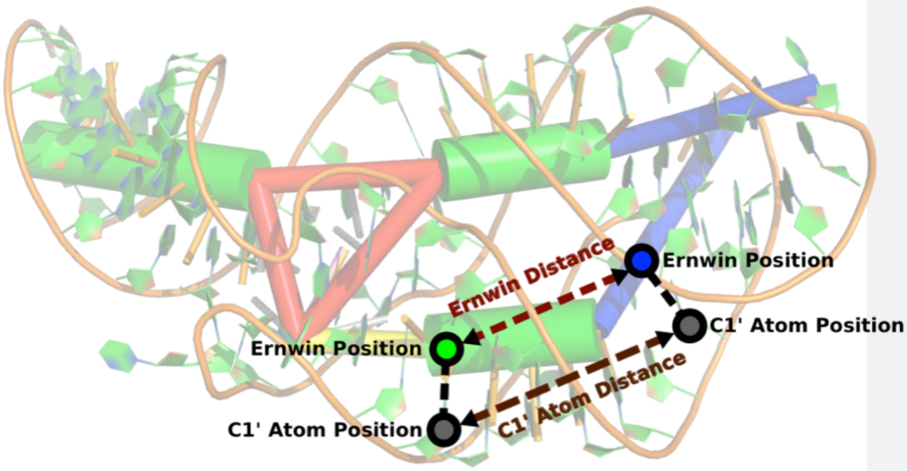


**S2 Fig 2. The inter-atom distances calculated using the Ernwin approximation vs. the real distances from the PDB structure (A-ribsowitch-adenine complex, PDB ID: 1Y26 [reference: Structural Basis for Discriminative Regulation of Gene Expression by Adenine- and Guanine-Sensing mRNAs]).** For each secondary structure, by default $10^5$ structures were sampled with Ernwin. Each sampled structure is part of the ensemble of structures described by the probability distribution of the energy function. Each structure corresponds to a single MCMC step where a new structure is proposed, its energy is evaluated and based on that is either accepted or rejected. Structures generated using Ernwin usually contain the exact specified secondary structure except in rare cases when 3D statistics are missing for a particular secondary structure element. In such cases, the nearest secondary structure fragment is used (this can happen in the case of e.g. interior loops with, for example, 15 unpaired nucleotides on one strand and 13 unpaired on the other). Structures generated by Rosetta are not checked to ensure they contain the proper secondary structure, but are strongly directed toward it with energy penalties for incorrectly paired nucleotides. Using Rosetta, each structure was annealed using 10000 MCMC steps and by default 30 thousand 3D structures were sampled for each secondary structure.
